# Supplementary material for: MAR-3D: Progressive Masked Auto-regressor for High-Resolution 3D Generation
Source: arXiv:2503.20519 source file (2025-04-20)
Supplement: Supplementary file 1 [file X_suppl.tex]

\clearpage
\setcounter{page}{1}
\maketitlesupplementary
Detailed network architecture specifications, training procedures, and inference protocols are provided in the supplementary material.
% , along with additional visualizations. For a comprehensive demonstration of our results, please visit our project page at \href{https://mar-3d.github.io/MAR-3D-Page/}{our anonymous link}.
\paragraph{Network Architectures}
We implement our network architecture in PyTorch. The Pyramid VAE backbone comprises a 16-layer encoder and 32-layer decoder, with a latent dimension of 64 and network width of 768. This asymmetric design enables better feature extraction and reconstruction capabilities. The MAR component adopts a Transformer-based encoder-decoder architecture, featuring 16 layers in both the encoder and decoder paths, 16 attention heads per layer, and an embedding dimension of 1024. This design choice facilitates effective modeling of long-range dependencies in 3D geometry. The MLP-based diffusion module consists of 6 layers with a width of 1024, which provides sufficient capacity for the denoising process while maintaining computational efficiency. For condition encoding, we leverage pre-trained vision transformers: DINOv2 ViT-g/14 and CLIP ViT-Large-Patch14. Prior to feeding images into the encoders, we resize all input images to a resolution of 224×224 pixels.
% These models are selected for their complementary strengths - DINOv2 excels at capturing fine-grained visual features and geometric relationships, while CLIP provides robust semantic understanding through its joint vision-language training. We extract features from the final attention layer of both models and project them to our model's embedding space through learnable linear layers.
\paragraph{Training and Inference Details}
Our MAR-LR and MAR-HR and trained parallel with the same training strategy using coarse and fine-grained data. Optimization
For training, we employ the AdamW optimizer with an initial learning rate of $1\times10^{-5}$, $\beta_1=0.9$, $\beta_2=0.99$, and $\varepsilon=1\times10^{-6}$. We adopt a two-stage learning rate schedule: first, a linear warm-up is applied for 5000 iterations, increasing the learning rate from $1\times10^{-11}$ to $1\times10^{-5}$, followed by a cosine annealing schedule that gradually decreases the learning rate to zero over 5000 iterations. This scheduling strategy helps stabilize early training while ensuring convergence in later stages.
During inference, the reverse denoising steps is set to 100. Auto-regressive steps are set to 64 for MAR-LR, taking 40 seconds, while MAL-HR used 32 steps, requiring 20 seconds.
\paragraph{Shape Variation}
Our method demonstrates the ability to generate diverse 3D meshes while maintaining fidelity to the input reference images. As shown in Fig.~\ref{fig:var}, given a single conditioning image (leftmost column), our approach can produce multiple plausible 3D mesh variations by sampling different random seeds. For both the cartoon fox and Mario character examples, the generated meshes preserve the key characteristics and style of the input while exhibiting meaningful variations in pose and subtle geometric details. All variations maintain coherent 3D structure and consistent proportions, suggesting that our method successfully learns to explore the latent space of plausible 3D shapes within the constraints defined by the input image. This variational capability is particularly valuable for content creation applications where users may want to generate multiple creative alternatives from a single reference.
\begin{figure}
\centering 
\includegraphics[width=0.48\textwidth]{var.pdf} 
\caption{\textbf{Shape variation of our MAR-3D}
We show side views of meshes generated from the same input condition image using different random seeds.}
\label{fig:var}
\end{figure}
\paragraph{More Ablation Study}
We conduct a quantitative evaluation study comparing our progressive MAR design with DiT. Results in Tab.~\ref{tab:ablation_supp} corroborate our findings from the Generation Ablations section in the main paper: our cascaded MAR architecture with condition augmentation outperforms the DiT structure, providing an efficient and effective approach for scaling up token resolution while maintaining model performance and computational efficiency.

\begin{table}
\centering
\begin{tabular}{l|ccc}
\hline
Setting &  F-Score $\uparrow$ & CD $\downarrow$ &NC$\uparrow$  \\
\hline
(a) & 0.901 & 0.553 & 0.755 \\
(b)& 0.834 & 0.786 & 0.721 \\
(c)& 0.855 & 0.687& 0.743 \\
(d)& 0.911 & 0.545 & 0.758 \\
(e)& 0.921 &0.411  &0.794 \\
(f) & 0.878 & 0.604 & 0.762 \\
(g) & 0.902 &0.435 &0.789 \\
\hline
(h) & 0.944 & 0.351 & 0.835 \\
\hline
\end{tabular}
\caption{\textbf{Ablation study of different components in our method.} Configurations (a) through (h) correspond to those presented in the Generation Ablations section of the main paper.}
\label{tab:ablation_supp}
\end{table}
